# Supplementary material for: Teleported free energy simulations
Source: arXiv:2610.40428 source file (2026-10-29)
Supplement: Supplementary file 1 [file appendix_floors.tex]

\section{Variance and dissipation floors}
\label{sec:floors}

Here we derive Eqs.~(M\ref{M-eq:chi2general})--(M\ref{M-eq:threshold}). The derivation uses only the identity~(\ref{eq:exact}) and therefore holds for any dynamics considered here, with or without flow and jumps, for both forms of the work and at any step size.

\paragraph*{Basin relation.} Let $\hat\pi_c$ be the probability that a trajectory ends in basin $\Omega_c$, and $\avg{\,\cdot\,|\,c}$ an average conditioned on this event. Integrating the second relation in Eq.~(\ref{eq:exact}) over $\Omega_c$ gives
\begin{equation}
\hat\pi_c\,\avg{e^{-\beta W}\,|\,c}=e^{-\beta\Delta F}\,\pi_c(B).
\label{eq:basin}
\end{equation}
Trajectories that end in basin $c$ must therefore carry, on average, a weight proportional to $\pi_c(B)/\hat\pi_c$. Under the conditions of Sec.~\ref{sec:local}, Eq.~(\ref{eq:basin}) implies $\hat\pi_c>0$ whenever $\pi_c(B)>0$, so that all ratios below are well defined.

\paragraph*{Variance floor.} Decomposing the second moment over final basins and using $\avg{X^2|c}\ge\avg{X|c}^2$ in each basin,
\begin{equation}
\avg{e^{-2\beta W}}=\sum_c\hat\pi_c\,\avg{e^{-2\beta W}\,|\,c}
\;\ge\;\sum_c\hat\pi_c\,\avg{e^{-\beta W}\,|\,c}^2
=e^{-2\beta\Delta F}\sum_c\frac{\pi_c(B)^2}{\hat\pi_c},
\end{equation}
where the last step uses Eq.~(\ref{eq:basin}). Dividing by $\avg{e^{-\beta W}}^2=e^{-2\beta\Delta F}$ yields Eq.~(M\ref{M-eq:chi2general}),
\begin{equation}
\frac{{\rm Var}\big[e^{-\beta W}\big]}{\avg{e^{-\beta W}}^2}\;\ge\;\sum_c\frac{\pi_c(B)^2}{\hat\pi_c}-1=\chi^2\big(\pi^B\big\|\hat\pi\big).
\label{eq:chi2proof}
\end{equation}
Equality holds if and only if $e^{-\beta W}$ is constant within each final basin: the floor is the between-basin part of the variance, which no dynamics inside the basins can remove. This is the coarse-grained version of the statement that importance weights cannot have a relative variance smaller than the $\chi^2$ divergence between target and sampled distributions~\cite{Doucet2022}.

\paragraph*{Dissipation floor.} By Jensen's inequality within each basin, $\avg{e^{-\beta W}|c}\ge e^{-\beta\avg{W|c}}$, so that Eq.~(\ref{eq:basin}) gives
$\avg{W\,|\,c}\ge\Delta F-\beta^{-1}\ln\big[\pi_c(B)/\hat\pi_c\big]$. Averaging with weights $\hat\pi_c$,
\begin{equation}
\beta\avg{W}-\beta\Delta F\;\ge\;\sum_c\hat\pi_c\ln\frac{\hat\pi_c}{\pi_c(B)}=D_{\rm KL}\big(\hat\pi\big\|\pi^B\big),
\label{eq:klproof}
\end{equation}
with equality if and only if $W$ is constant within each final basin.

\paragraph*{Continuous escorts.} A continuous flow generates a homeomorphism of phase space at each step. If, in addition, neither the flow nor the physical dynamics carries trajectories across the barriers during the process, every trajectory ends in the basin where it started, and $\hat\pi_c=\pi_c(A)$. Equations~(\ref{eq:chi2proof}) and~(\ref{eq:klproof}) then reduce to Eq.~(M\ref{M-eq:floor}),
\begin{equation}
\frac{{\rm Var}\big[e^{-\beta W}\big]}{\avg{e^{-\beta W}}^2}\ge\chi^2\big(\pi^B\big\|\pi^A\big),\qquad
\beta\avg{W}-\beta\Delta F\ge D_{\rm KL}\big(\pi^A\big\|\pi^B\big),
\end{equation}
which depend only on the equilibrium basin weights at the two end points and not on $\mathbf u$. For example, for the model of Fig.~1 of the main text with $h=2$, $\pi_R(0)=1.3\times10^{-5}$ and $\pi_R(1)=1/2$: trajectories starting on the right must carry weights about $0.5/(1.3\times10^{-5})\approx4\times10^4$ times the mean, and $\chi^2\simeq(1/2)^2/\pi_R(0)\approx2\times10^4$, as measured in Fig.~2.

\paragraph*{Minimal teleportation activity.} Without barrier crossings by the flow or the physical dynamics, basin occupations change only through inter-basin jumps. Let $n_c^{\rm in}$ and $n_c^{\rm out}$ be the numbers of jumps into and out of basin $c$ along a trajectory, and $n=\tfrac12\sum_c(n_c^{\rm in}+n_c^{\rm out})$ the number of inter-basin jumps. Then $\hat\pi_c-\pi_c(A)=\avg{n_c^{\rm in}}-\avg{n_c^{\rm out}}$, and
\begin{equation}
\tfrac12\sum_c\big|\hat\pi_c-\pi_c(A)\big|\;\le\;\tfrac12\sum_c\big(\avg{n_c^{\rm in}}+\avg{n_c^{\rm out}}\big)=\avg{n},
\end{equation}
which is Eq.~(M\ref{M-eq:activity}). By Eq.~(\ref{eq:chi2proof}), zero variance requires $\hat\pi=\pi^B$, hence $\avg{n}\ge d_{\rm TV}(\pi^A,\pi^B)$, Eq.~(M\ref{M-eq:threshold}). In the two-basin model the perfect teleport saturates this bound (Sec.~\ref{sec:toy}).
